# Supplementary material for: Geometry-aware Active Learning of Spatiotemporal Dynamic Systems
Source: arXiv:2504.19012 source file (2025-05-01)
Supplement: Supplementary file 1 [file Appendix.tex]

\onecolumn
\section*{Symbols and Description}
\begin{longtable}{p{.20\textwidth} | p{.80\textwidth}} 
	Symbol & Description\\
	\hline
	$\mathbb{N}$ & Set of natural numbers $\{0,1,2,3,\ldots\}$\\
	$\mathbb{N}^*$ & Set of positive natural numbers $\{1,2,3,\ldots\}$\\
  $\mathcal{X}_\text{tr}$ & Set of spatial locations $\mathcal{X}_\text{tr}=\{\vect{x}_1,\vect{x}_2,\dots,\vect{x}_{N_s}\}$\\
  $\mathcal{X}^*$ & Set of spatial locations in test set\\
  $\mathcal{X}_{n(-i)}$ & Set of spatial locations excluding $\vect{x}_i$\\
	$\mathcal{T}_\text{tr}$ & Set of time points $\mathcal{T}_\text{tr}=\{t_1,t_2,\dots,t_{N_t}\}$\\
	$\mathcal{T}^*$ & Set of time points in test set\\
	$u(\vect{x},t)$ & Random variable describing the underlying system dynamics at location $\vect{x}$ and time $t$\\
	$\hat{\mu}_{-\vect{x}_i}(\vect{x}_i,t_j)$ & Prediction based on the training data excluding samples at spatial location $\vect{x}_i$\\
	$y(\vect{x},t)$ & Observed value of the random variable $u(\vect{x},t)$\\
  $\vect{y}_{(i)}$ & Combined vector $\left[y(\vect{x}_i,t_j)\right]_{t_j\in \mathcal{T}_\text{tr}}$\\
	$\vect{y}_n$ & Abbreviation for vector $[\vect{y}_{(i)},\vect{y}_{n(-i)}]$\\
  $\vect{y}_{n(-i)}$ & Observations at spatial locations in $\mathcal{X}_{n(-i)}$\\
	$\left( \Sigma_{n,N_\text{t}}^{-1} \mathbf{y}_{n} \right)_{(1_i, \cdot)N_\text{t}}$ & Sub-vector of $ \Sigma_{n,N_\text{t}}^{-1} \mathbf{y}_{n} $ for $i$-th spatial location\\
	$\vect{r} = \vect{x} - \vect{x}'$ & Spatial displacement vector\\
	$\mathcal{K}$ & Kernel operator\\
	$\mathcal{K}(\cdot,\cdot)$ & Kernel function with inputs\\
  $\mathcal{K}^*$ & Test-training matrix block of $\mathcal{K}$\\
	$\mathcal{K}^{**}$ & Test-test matrix block of $\mathcal{K}$\\
  $1_i$ & Unit indicator for $i^\text{th}$ element\\
  $\mathcal{K}_{(1_i, n - 1_i),N_\text{t}}$ & Cross-covariance between location $i$ and other locations\\
  $\mathcal{K}_{(1_i, 1_i),N_\text{t}}$ & Self-covariance at location $i$\\
  $\Sigma$ & Covariance matrix of kernel $\mathcal{K}$\\
  $\Sigma_{n(-i)}$ & Covariance matrix of $\mathcal{K}_\text{s}$ based on the training data excluding sample $\vect{x}_i$\\
	$\text{tr}$ & Subscript denoting related training dataset\\
	$\text{s}$ & Subscript denoting spatial kernel $\mathcal{K}_{\text{s}}$\\
	$\text{t}$ & Subscript denoting temporal kernel $\mathcal{K}_{\text{t}}$\\
	$\text{st}$ & Subscript denoting spatiotemporal kernel $\mathcal{K}_{\text{st}}$\\
	$\epsilon$ & Subscript denoting measurement noise\\
	$\Omega$ & A compact set in Euclidean space\\
	$\partial\Omega$ & Boundary of domain $\Omega$\\
  $\vect{n}_{\partial\Omega}$ & Normal vector on $\partial\Omega$\\
  $|\Omega_i|$ & Area of $i_\text{th}$ Voronoi cell\\
	$\vect{s}$ & Fourier frequency vector\\
	$\mu$ & Positive finite measure on $\Omega$\\
	$f(\mathbf{x})$ or $\mathbf{f}$ & Vector of latent function values, $\mathbf{f} = (f(\mathbf{x}_1), \ldots, f(\mathbf{x}_n))^\top$\\
	$\Delta$ & Laplacian operator\\
	$S(\cdot)$ & Spectral density function\\
	$(\lambda_j, \phi_j)$ & Laplacian eigenvalue-eigenvector  pair under index $j$\\
	$\delta_{ij}$ & Kronecker delta, 1 if $i=j$, 0 otherwise.\\
	$l(\cdot, \cdot)$ & Laplacian function\\
	$a$ & Generic constant\\
	$M$ & Manifold geometry with $N$ discretized vertices\\
  $N(i)$ & Set of neighboring vertices connected to vertex $i$\\
  $N_t$ & Number of temporal samples per location\\
  $\alpha_{ij},\beta_{ij}$ & Angle opposite edge $(i,j)$\\
  $\vect{\theta}$ & Parameters' set $\vect{\theta}=\{l_{\text{s}}, \sigma_m, \sigma_{\epsilon,\text{s}}, l_{\text{t}}, \sigma_a, \sigma_{\epsilon,\text{t}}\}$\\
  $\epsilon(\vect{x},t)$ & Spatiotemporal noise term\\
  $\sigma_m$ & Spatial kernel scaling parameter\\
  $\sigma_{\epsilon,\text{s}}$ & Spatial noise level\\
  $\hat{\sigma}^2_{n;\epsilon,\text{s}}$ & Estimated spatial noise level\\
	$\sigma_a$ & Temporal kernel scaling parameter\\
	$\sigma_{\epsilon,\text{t}}$ & Temporal noise level\\
  $\hat{\vect{\nu}}$ & Gaussian Process prediction uncertainty\\
  $\hat{\sigma}_n(\vect{x})$ & Prediction uncertainty at $\vect{x}$ given $n$ spatial measured data\\
	$d$ & Dimension (2 for surface manifolds)\\
	$\Gamma$ & Gamma function\\
	$\nu$ & Smoothness parameter\\
  $l_{\text{s}}$ & Spatial length-scale parameter\\
  $l_{\text{t}}$ & Temporal length-scale parameter\\
	$\operatorname{vec}(\cdot)$ & Vectorization operator that stacks matrix columns into a single column vector\\ 
	$\operatorname{vec}(\cdot)^{-1}$ & Inverse operation of $\operatorname{vec}(\cdot)$\\
  $\operatorname{diag}(\cdot)$ & Diagonal extraction operator\\
	$d_g(\vect{x},\vect{x}_i)$ & Geodesic distance between $\vect{x}$ and $\vect{x}_i$\\
	$\alpha_{n,1}$ & Weight for space-filling criterion\\
	$\alpha_{n,2}$ & Weight for uncertainty-based criterion\\
  $\gamma$ & Ratio of $\alpha_{n,1}/\alpha_{n,2}$\\
	$\hat{\tau}_{n,\text{cv}}^2$ & Leave-one-out cross-validation error from model trained on $n$ spatial samples\\
	\hline
	\caption{Symbols and descriptions}
\end{longtable}
% \twocolumn
